# Supplementary material for: Topological Autoencoders
Source: arXiv:1906.00722 source file (2021-05-31)
Supplement: Supplementary file 1 [file supp_results.tex]

\begin{tiny}
\setlength{\tabcolsep}{3pt}
\begin{tabular}{llrrrrrrrrrr}
\toprule
 Data set &   Method & $\dkl_{0.001}$ & $\dkl_{0.01}$ &  $\dkl_{0.1}$ &   $\dkl_{1}$ & $\dkl_{10}$ & $\ell$-Cont & $\ell$-MRRE &  $\ell$-Trust & $\ell$-RMSE & Data MSE \\
\midrule
%%%%%%%%%%%%%%%%%%%%%%%%%%%%
% SPHERE DATASET 
%%%%%%%%%%%%%%%%%%%%%%%%%%%%
\multirow{6}*{\data{Spheres}}     &	Isomap            &         0.53095 $\pm$ 0.01929 &        0.18096 $\pm$ 0.02547 &       \second{0.42048} $\pm$ 0.00559 &      \second{0.00881} $\pm$ 0.00020 &       \second{0.00009} $\pm$ 0.00000 &  \second{0.79027} $\pm$ 0.00244 &  \second{0.24573} $\pm$ 0.00158 &       \second{0.67643} $\pm$ 0.00323 &  10.37188 $\pm$ 0.22856 &                       --  \\
 & PCA               &         \first{0.22445} $\pm$ 0.00691 &        0.33231 $\pm$ 0.00552 &       0.65121 $\pm$ 0.00256 &      0.01530 $\pm$ 0.00010 &       0.00016 $\pm$ 0.00000 &  0.74740 $\pm$ 0.00140 &  0.29402 $\pm$ 0.00108 &       0.62557 $\pm$ 0.00066 &  11.76482 $\pm$ 0.01460 &       0.96103 $\pm$ 0.00029 \\
 & TSNE              &         \second{0.22794} $\pm$ 0.00722 &        \second{0.15228} $\pm$ 0.00805 &       0.52722 $\pm$ 0.03261 &      0.01271 $\pm$ 0.00058 &       0.00013 $\pm$ 0.00001 &  0.77300 $\pm$ 0.00513 &  \first{0.21740} $\pm$ 0.00472 &       \first{0.67862} $\pm$ 0.00474 &   \first{8.05018} $\pm$ 0.11057 &                       -- \\
 & UMAP              &         0.24752 $\pm$ 0.01917 &        0.15687 $\pm$ 0.00599 &       0.61326 $\pm$ 0.00752 &      0.01658 $\pm$ 0.00028 &       0.00018 $\pm$ 0.00000 &  0.75153 $\pm$ 0.00360 &  0.24968 $\pm$ 0.00094 &       0.63483 $\pm$ 0.00185 &   \second{9.27009} $\pm$ 0.03417 &                       --  \\
 & AE           &         0.28432 $\pm$ 0.02165 &        0.56571 $\pm$ 0.02864 &       0.74588 $\pm$ 0.04323 &      0.01664 $\pm$ 0.00115 &       0.00017 $\pm$ 0.00001 &  0.60663 $\pm$ 0.01685 &  0.34918 $\pm$ 0.00903 &       0.58843 $\pm$ 0.00475 &  13.33061 $\pm$ 0.05198 &       0.81545 $\pm$ 0.00106 \\
 & TopoAE &         0.62765 $\pm$ 0.05415 &        \first{0.08504} $\pm$ 0.01270 &       \first{0.32572} $\pm$ 0.02050 &      \first{0.00694} $\pm$ 0.00055 &       \first{0.00007} $\pm$ 0.00001 &  \first{0.82200} $\pm$ 0.01813 &  0.27239 $\pm$ 0.01108 &       0.65775 $\pm$ 0.01428 &  13.45753 $\pm$ 0.04177 &       0.86812 $\pm$ 0.00074 \\
\midrule
 %%%%%%%%%%%%%%%%%%%%%%%%%%%%
 % Fashion MNIST
 %%%%%%%%%%%%%%%%%%%%%%%%%%%%
\multirow{5}*{\data{Fashion-MNIST}} & PCA               &         0.22559 $\pm$ 0.00011 &        \first{0.35594} $\pm$ 0.00011 &       \first{0.05205} $\pm$ 0.00004 &      \first{0.00069} $\pm$ 0.00000 &       \first{0.00001} $\pm$ 0.00000 &  0.96777 $\pm$ 0.00001 &  0.05744 $\pm$ 0.00001 &       0.91681 $\pm$ 0.00003 &   \first{9.05121} $\pm$ 0.00041 &       0.18439 $\pm$ 0.00000 \\
& TSNE              &         \first{0.03516} $\pm$ 0.00226 &        0.40477 $\pm$ 0.01251 &       0.07095 $\pm$ 0.00962 &      0.00198 $\pm$ 0.00026 &       0.00002 $\pm$ 0.00000 &  0.96731 $\pm$ 0.00268 &  \first{0.01962} $\pm$ 0.00073 &       \second{0.97405} $\pm$ 0.00070 &  41.25460 $\pm$ 0.53671 &                       -- \\
& UMAP              &         \second{0.05069} $\pm$ 0.00238 &        0.42362 $\pm$ 0.00609 &       0.06491 $\pm$ 0.00161 &      0.00163 $\pm$ 0.00005 &       0.00002 $\pm$ 0.00000 &  \first{0.98126} $\pm$ 0.00016 &  0.02867 $\pm$ 0.00034 &       0.95874 $\pm$ 0.00060 &  \second{13.68933} $\pm$ 0.02896 &                       -- \\
& AE           &         0.17177 $\pm$ 0.13603 &        0.47798 $\pm$ 0.09567 &       0.06791 $\pm$ 0.00700 &      0.00125 $\pm$ 0.00017 &       0.00001 $\pm$ 0.00000 &  0.96849 $\pm$ 0.00372 &  \second{0.02562} $\pm$ 0.00217 &       \first{0.97418} $\pm$ 0.00119 &  20.70674 $\pm$ 3.56861 &       0.10197 $\pm$ 0.00222 \\
& TopoAE &         0.11039 $\pm$ 0.02948 &        \second{0.39204} $\pm$ 0.03264 &       \second{0.05353} $\pm$ 0.00959 &      \second{0.00100} $\pm$ 0.00015 &       \second{0.00001} $\pm$ 0.00000 &  \second{0.97998} $\pm$ 0.00194 &  0.03156 $\pm$ 0.00253 &       0.95612 $\pm$ 0.00391 &  20.49122 $\pm$ 0.93206 &       0.12071 $\pm$ 0.00238 \\
 \midrule
 %
 % MNIST
 %
 \multirow{5}*{\data{MNIST}} & PCA               &         0.16754 $\pm$ 0.00051 &        0.38876 $\pm$ 0.00146 &       0.16301 $\pm$ 0.00059 &   0.00160 $\pm$ 0.00001 &        0.00002 $\pm$ 0.00000 &  0.90084 $\pm$ 0.00016 &  0.16582 $\pm$ 0.00022 &       0.74546 $\pm$ 0.00048 &  \first{13.17437} $\pm$ 0.00216 &       0.22269 $\pm$ 0.00002 \\
& TSNE              &         \first{0.03767} $\pm$ 0.00140 &        \first{0.27695} $\pm$ 0.05266 &       \second{0.13266} $\pm$ 0.02362 &      0.00214 $\pm$ 0.00041 &       0.00002 $\pm$ 0.00000 &  0.92101 $\pm$ 0.00288 &  \first{0.03953} $\pm$ 0.00129 &       \first{0.94624} $\pm$ 0.00147 &  22.89261 $\pm$ 0.24373 &                       -- \\
&  UMAP              &         \second{0.07214} $\pm$ 0.00091 &        \second{0.32063} $\pm$ 0.00320 &       0.14568 $\pm$ 0.00207 &      0.00234 $\pm$ 0.00004 &       0.00003 $\pm$ 0.00000 &  \first{0.93992} $\pm$ 0.00066 &  \second{0.05109} $\pm$ 0.00022 &       \second{0.93770} $\pm$ 0.00039 &  \second{14.61535} $\pm$ 0.04332 &                       -- \\
&  AE           &         0.44690 $\pm$ 0.08540 &        0.61993 $\pm$ 0.11742 &       \second{0.15542} $\pm$ 0.02203 &      0.00156 $\pm$ 0.00023 &       \second{0.00002} $\pm$ 0.00000 &  0.91293 $\pm$ 0.00564 &  0.05828 $\pm$ 0.00353 &       0.93699 $\pm$ 0.00262 &  18.18105 $\pm$ 0.21459 &       0.13732 $\pm$ 0.00160 \\
& TopoAE  &         0.32427 $\pm$ 0.03312 &        0.34069 $\pm$ 0.03056 &       \first{0.11012} $\pm$ 0.01069 &      \first{0.00114} $\pm$ 0.00010 &       \first{0.00001} $\pm$ 0.00000 &  \second{0.93210} $\pm$ 0.00132 &  0.05553 $\pm$ 0.00044 &       0.92844 $\pm$ 0.00142 &  19.57784 $\pm$ 0.01812 &       0.13884 $\pm$ 0.00066 \\
 \midrule
 %
 % CIFAR
 %
\multirow{5}*{\data{CIFAR}} & PCA               &         0.27320 $\pm$ 0.00014 &        \second{0.59073} $\pm$ 0.00004 &       \second{0.01961} $\pm$ 0.00001 &      \first{0.00023} $\pm$ 0.00000 &       \first{0.00000} $\pm$ 0.00000 &  \first{0.93130} $\pm$ 0.00000 &  0.11921 $\pm$ 0.00005 &       0.82117 $\pm$ 0.00002 &  \first{17.71567} $\pm$ 0.00084 &       0.14816 $\pm$ 0.00000 \\
& TSNE              &         \first{0.04451} $\pm$ 0.00222 &        0.62733 $\pm$ 0.01427 &       0.03014 $\pm$ 0.00333 &      0.00073 $\pm$ 0.00007 &       0.00001 $\pm$ 0.00000 &  0.90300 $\pm$ 0.00611 &  \first{0.10265} $\pm$ 0.00242 &       \second{0.86325} $\pm$ 0.00151 &  \second{25.61099} $\pm$ 0.11551 &                       -- \\
&  UMAP              &        \second{0.06934} $\pm$ 0.00202 &        0.61673 $\pm$ 0.00052 &       0.02562 $\pm$ 0.00019 &      0.00050 $\pm$ 0.00001 &       0.00001 $\pm$ 0.00000 &  0.92045 $\pm$ 0.00013 &  0.12680 $\pm$ 0.00028 &       0.81668 $\pm$ 0.00019 &  33.57785 $\pm$ 0.00796 &                       -- \\
&  AE           &         0.37737 $\pm$ 0.06507 &        0.66834 $\pm$ 0.02992 &       0.03458 $\pm$ 0.00448 &      0.00062 $\pm$ 0.00021 &       0.00001 $\pm$ 0.00000 &  0.85072 $\pm$ 0.00429 &  0.13204 $\pm$ 0.00316 &       \first{0.86359} $\pm$ 0.00442 &  36.26827 $\pm$ 0.56159 &       0.14030 $\pm$ 0.00190 \\
&  TopoAE  &         0.20877 $\pm$ 0.00951 &        \first{0.55642} $\pm$ 0.00412 &       \first{0.01879} $\pm$ 0.00051 &      \second{0.00031} $\pm$ 0.00002 &       \second{0.00000} $\pm$ 0.00000 &  \second{0.92691} $\pm$ 0.00100 &  \second{0.10809} $\pm$ 0.00210 &       0.84514 $\pm$ 0.00359 &  37.85914 $\pm$ 0.03303 &       0.13975 $\pm$ 0.00171 \\
\bottomrule
\end{tabular}
\end{tiny}
