# Supplementary material for: Topological Autoencoders
Source: arXiv:1906.00722 source file (2021-05-31)
Supplement: Supplementary file 2 [file table_supp.tex]

\begin{tabular}{llrrrrr}
\toprule
 Data set &              Method &  $\dkl_{0.01}$ &  $\dkl_{0.1}$ &   $\dkl_{1}$ &  MRRE &   RMSE \\

\midrule
    &               UMAP &                    \textit{0.025075} &                   \textit{0.012997} &                  0.001633 &        \textit{0.017706} &   13.148808 \\
    \multirow{6}*{\data{SCurve}} &            AE &                    0.056538 &                   0.019945 &                  \textit{0.001265} &        0.038442 &    1.582880 \\
             &                PCA &                    0.032992 &                   0.020228 &                  \textbf{0.000768} &        0.100973 &    \textbf{0.709067} \\
             &               TSNE &                    0.036500 &                   0.032353 &                  0.001997 &        0.038390 &   51.735474 \\
             &             Isomap &                    \textbf{0.016870} &                   \textbf{0.012698} &                  0.001571 &        \textbf{0.014569} &    2.509537 \\
             &  TopoAE (proposed) &                    0.078835 &                   0.028975 &                  0.001398 &        0.044565 &    \textit{0.986490} \\
            
\bottomrule
\end{tabular}
